# Supplementary material for: Homomorphically encrypted gradient descent algorithms for quadratic programming
Source: arXiv:2309.01559 source file (2023-09-04)
Supplement: Supplementary file 1 [file appendix.tex]

\section{Implementation}
\label{appendix:implementation}
For the numerical examples presented here we used our own Python
wrapper of the Microsoft SEAL \cite{SEAL21} C++ library and run the
code in an Intel Xeon E5-1620 with 24GB of RAM running Debian 11. All
the code for the implementation of the numerical results are available
on Github:
\begin{itemize}
\item[] Wrapper: https://github.com/b3rt01ac3/pSEAL
\item[] Gradient descent: https://github.com/b3rt01ac3/agd-he
\end{itemize}
